# Supplementary material for: Can't Touch This: Real-Time, Safe Motion Planning and Control for Manipulators Under Uncertainty
Source: arXiv:2301.13308 source file (2023-11-01)
Supplement: Supplementary file 1 [file 11_appendix_F.tex]

\section{Comparison of Robust Input Bound}
\label{app:input_bound_comparison}
\methodname's robust input (given in \eqref{eq:robust_input}) is inspired by \cite{giusti2016bound, giusti2017efficient}.
We claim that the proposed controller improves on these published controllers because it achieves the same uniform bound with a smaller robust input bound.
From \cite[Thm. 1, (10)]{giusti2016bound}, the robust input given in previous work is
\begin{equation}
    \robv(\qA(t), \Delta_0, [\Delta]) = - 
    \Big( 
    \kappa(t) \norm{\wmax(\qA(t),\Delta_0,[\Delta])}
    + \phi(t)
    \Big) \robr(t),
    \label{eq:giusti_robust_input}
\end{equation}
where $\kappa$ and $\phi$ are positive increasing functions with $\kappa_P \geq 1$ and $\phi_P \geq 1$ as their respective minimums, and $\wmax(\qA(t),\Delta_0,[\Delta])$ as in \eqref{eq:cond_wmax}.
With this choice of robust input, \cite[Thm. 1]{giusti2016bound} proves that the trajectories of $r$ are ultimately uniformly bounded by $\norm{r(t)} \leq \frac{1}{\kappa_P}\sqrt{\frac{\sigM}{\sigm}} \quad \forall t \geq t_1,$
% \begin{equation}
%     \norm{r(t)} \leq \frac{1}{\kappa_P}\sqrt{\frac{\sigM}{\sigm}} \quad \forall t \geq t_1
%     \label{eq:giusti_ultimate_bound}
% \end{equation}
where $t_1$ is some finite time.
In the context of Rem. \ref{rem:combining_traj}, this bound holds for all time if \eqref{eq:giusti_robust_input} were used in the current framework.
This uniform bound can be made identical to \eqref{eq:ultimate_bound} by choosing $\kappa_P = \sqrt{\frac{\sigM}{2\roblevel}}$. 
% which yields
% \begin{equation}
%     \frac{1}{\kappa_P}\sqrt{\frac{\sigM}{\sigm}} = 
%     \sqrt{\frac{2\roblevel}{\sigM}}\sqrt{\frac{\sigM}{\sigm}} = \sqrt{\frac{2\roblevel}{\sigm}}
% \end{equation}
% as desired.

To bound the magnitude of the robust input similarly to App. \ref{app:robust_input_bound}, note
\begin{equation}
    \abs{\robv(\qA(t), \Delta_0, [\Delta])}_j = \Big( 
    \kappa(t) \norm{\wmax(\qA(t),\Delta_0,[\Delta])}
    + \phi(t)
    \Big) \abs{\robr_j(t)}.
\end{equation}
The smallest possible bound on $\abs{\robr_j(t)}$ is given by $\norm{r(t)} \leq \frac{1}{\kappa_P}\sqrt{\frac{\sigM}{\sigm}}$, which yields $\abs{\robr_j(t)} \leq \norm{r(t)} \leq \frac{1}{\kappa_P}\sqrt{\frac{\sigM}{\sigm}}$.
Defining $\wmax(\pzgreek{*}) = \wmax(\pzi{\qA},\nomparams,\intparams)$ as in \eqref{eq:pz_w_max}, we have
\begin{equation}
    \label{eq:giusti_input_bound}
    \abs{\robv(\qA(t), \Delta_0, [\Delta])}_j \leq \Big( 
    \kappa(t) \norm{\wmax(\pzgreek{*})}
    + \phi(t)
    \Big) \frac{1}{\kappa_P}\sqrt{\frac{\sigM}{\sigm}}
\end{equation}
for all $t \in \pz{T_i}$.
Next, we show that a lower bound on the right hand side of this equation (i.e., a lower bound on the robust input bound) is larger than the robust input bound \eqref{eq:pz_robust_input_bound}.

Using the properties of $\kappa$ and $\phi$,
\begin{equation}
    \Big( 
    \kappa_P \norm{\wmax(\pzgreek{*})}
    \Big) \frac{1}{\kappa_P}\sqrt{\frac{\sigM}{\sigm}}
    \leq \Big( 
    \kappa(t) \norm{\wmax(\pzgreek{*})}
    + \phi(t)
    \Big) \frac{1}{\kappa_P}\sqrt{\frac{\sigM}{\sigm}}.
\end{equation}
Cancelling terms on the left hand side gives
\begin{equation}
    \norm{\wmax(\pzgreek{*})}\sqrt{\frac{\sigM}{\sigm}}
    \leq \Big( 
    \kappa(t) \norm{\wmax(\pzgreek{*})}
    + \phi(t)
    \Big) \frac{1}{\kappa_P}\sqrt{\frac{\sigM}{\sigm}}.
\end{equation}
The robust input bound for \eqref{eq:giusti_robust_input} is larger than $\norm{\wmax(\pzgreek{*})}\sqrt{\frac{\sigM}{\sigm}}$.

We compare this value to ARMOUR's robust input bound in \eqref{eq:pz_robust_input_bound}.
Under what conditions is \eqref{eq:pz_robust_input_bound} smaller, i.e. 
\begin{equation}
    \frac{\alpha_c \epsilon(\sigma_M - \sigma_m) + \norm{\wmax(\pzgreek{*})} + \wmax(\pzgreek{*})_j}{2}
    \stackrel{?}{\leq}
    \norm{\wmax(\pzgreek{*})}\sqrt{\frac{\sigM}{\sigm}}.
\end{equation}
This relation depends on the user-specified constants $\alpha_c$ and $\epsilon$ and $\sigM$ and $\sigm$, but generally the following are true.
First, $\sigM \geq \sigm$ by definition, and usually $\sigM$ is much larger than $\sigm$.
Second, $\epsilon$ is the user-specified uniform bound and a small constant is desired to minimize tracking error.
Third, the $j$\ts{th} component of the worst case disturbance $\wmax(\pzgreek{*})_j$ is smaller than $\norm{\wmax(\pzgreek{*})}$.
Therefore, ignoring the term involving $\epsilon$ (which is small), ARMOUR's robust input bound \eqref{eq:pz_robust_input_bound} is smaller than \eqref{eq:giusti_input_bound} by at least a factor of $\sqrt{\frac{\sigM}{\sigm}}$.

To give an idea of the differences, consider the Kinova Gen3 robot as reported in Sec. \ref{sec:experiments:alg_implementation}.: $\alpha_c = 1$, $\epsilon = 0.049089$, $\sigM = 18.2726$, and $\sigm = 8.2993$.
Plugging in yields
\begin{equation}
    \frac{\alpha_c \epsilon(\sigma_M - \sigma_m) + \norm{\wmax(\pzgreek{*})} + \wmax(\pzgreek{*})_j}{2} \leq 0.4895 + \norm{\wmax(\pzgreek{*})},
\end{equation}
and 
\begin{equation}
    \norm{\wmax(\pzgreek{*})}\sqrt{\frac{\sigM}{\sigm}} = 1.48380\norm{\wmax(\pzgreek{*)}}.
\end{equation}
% In our computations, $\norm{\rho(*)}$ is on average around $17$Nm, so \pat{update number!}
